# Supplementary material for: Look Back to Move Forward: Learning to Revisit for Agentic Compositional Image Generation
Source: arXiv:2610.16224 source file (2026-10-12)
Supplement: Supplementary file 1 [file appendix_dependencies.tex]

\RequirePackage{graphicx,float,booktabs,array,tabularx,threeparttable}
\RequirePackage{amsmath,amssymb,algorithm,algpseudocode,listings}
\RequirePackage{tikz,needspace,etoolbox,fix-cm}
\RequirePackage[most]{tcolorbox}
\let\AppOriginalTTDefault\ttdefault
\RequirePackage{inconsolata,xurl}
\let\ttdefault\AppOriginalTTDefault
