# Supplementary material for: Look Back to Move Forward: Learning to Revisit for Agentic Compositional Image Generation
Source: arXiv:2610.16224 source file (2026-10-12)
Supplement: Supplementary file 2 [file appendix_styles.tex]

\RequirePackage{bookmark}
\usetikzlibrary{arrows.meta,calc,backgrounds}
\definecolor{appInk}{HTML}{243442}
\definecolor{appBlue}{HTML}{50799A}
\definecolor{appAmber}{HTML}{A87E36}
\definecolor{appGreen}{HTML}{448672}
\definecolor{appViolet}{HTML}{7A7095}
\definecolor{appMuted}{HTML}{667380}
\definecolor{appRule}{HTML}{D3DCE4}
\definecolor{appTableHead}{HTML}{E8EDFB}
\definecolor{appTableGroup}{HTML}{F6F7FA}
\definecolor{appBoxTeal}{HTML}{147D83}
\definecolor{appBoxInk}{HTML}{16324A}
\newtcolorbox{appbox}[2][appBoxTeal]{enhanced,breakable,
 colback=#1!5!white,colframe=#1!45!white,colbacktitle=#1!12!white,
 coltitle=appBoxInk,fonttitle=\bfseries,boxrule=.45pt,arc=1.4mm,
 title={#2},left=7pt,right=7pt,top=5pt,bottom=5pt,
 toptitle=4pt,bottomtitle=4pt,before skip=7pt,after skip=7pt,
 fontupper=\small}
\newtcblisting{appcode}[2][appBoxTeal]{enhanced,listing only,
 colback=#1!4!white,colframe=#1!45!white,colbacktitle=#1!12!white,
 coltitle=appBoxInk,fonttitle=\bfseries,title={#2},boxrule=.45pt,
 arc=1.4mm,left=7pt,right=7pt,top=5pt,bottom=5pt,
 before skip=7pt,after skip=7pt,
 listing options={basicstyle=\ttfamily\fontsize{8.5}{10.5}\selectfont,
 columns=fullflexible,breaklines=true,breakatwhitespace=false,
 keepspaces=true,showstringspaces=false,frame=none,aboveskip=0pt,
 belowskip=0pt,xleftmargin=0pt,xrightmargin=0pt}}
\newif\ifappdraftnotes
\appdraftnotestrue
\providecommand{\appnote}[1]{\ifappdraftnotes
 \begin{appbox}[appAmber]{Pending source material}#1\end{appbox}\fi}
\providecommand{\AppBookmark}[3]{} %
\providecommand{\AppActivateFormatting}{%
 \renewcommand{\ttdefault}{zi4}%
 \renewcommand{\tabularxcolumn}[1]{>{\raggedright\arraybackslash}p{##1}}%
}
\lstset{basicstyle=\ttfamily\fontsize{8.5}{10.5}\selectfont,
 columns=fullflexible,breaklines=true,keepspaces=true,showstringspaces=false}
\tikzset{
 appfigure/.style={x=1cm,y=-1cm,
 every node/.style={font=\sffamily\fontsize{8.3}{10}\selectfont,
 text=appInk,inner sep=0pt}},
 appedge/.style={-{Stealth[length=1.55mm,width=1.0mm]},
 draw=appMuted,line width=.65pt},
 appdetail/.style={draw=appMuted!70,line width=.45pt,densely dotted},
 appmeta/.style={font=\sffamily\fontsize{8}{9.5}\selectfont,text=appInk!78!white},
 appfigtitle/.style={font=\sffamily\bfseries\fontsize{9.1}{10.5}\selectfont},
 appchip/.style={rounded corners=1mm,fill=white,draw=appRule,
 line width=.4pt,inner xsep=4pt,inner ysep=2.4pt},
 apppanel/.style={rounded corners=1.7mm,line width=.4pt}}
